# Supplementary material for: ARBERT & MARBERT: Deep Bidirectional Transformers for Arabic
Source: arXiv:2101.01785 source file (2021-06-07)
Supplement: Supplementary file 1 [file Table_SI_2_Colum.tex]

\begin{table*}[H]
\centering

\begin{adjustbox}{width=\columnwidth}
{
\footnotesize
\begin{tabular}{lcclccc||lcclccc} 
\toprule
\multirow{2}{*}{\textbf{Data (\#classes)} } & \multirow{2}{*}{\textbf{SOTA} }     & \multirow{2}{*}{\textbf{Metric} } & \multirow{2}{*}{\textbf{LM} } & \multicolumn{3}{c}{\textbf{TEST} }      &   \\ 
\cline{5-7}
     &      &    && \textbf{Acc.}& \textbf{F1}  & \textbf{F\textsubscript{1}\textsuperscript{\textit{PN}}}  &  &      &    && \textbf{Acc.}& \textbf{F1}  & \textbf{F\textsubscript{1}\textsuperscript{\textit{PN}}}  \\ 
\toprule
\multirow{6}{*}{ArSAS (3) CAMel}    & \multirow{6}{*}{92\textsuperscript{$\star$} } & \multirow{6}{*}{F\textsubscript{1}\textsuperscript{\textit{PN}} }   
    & mBERT   & 89.65  & 88.67  & 87.50      & \multirow{6}{*}{ASTD (3) CAMel}     & \multirow{6}{*}{73\textsuperscript{$\star$} } & \multirow{6}{*}{F\textsubscript{1}\textsuperscript{\textit{PN}} }   
    & mBERT   & 59.54  & 55.15  & 67.00      \\
    
     &      &    &XLM-R\textsubscript{Base}       & 91.76  & 91.04  & 90.00      \\  &      &    &XLM-R\textsubscript{Base}       & 63.96  & 60.71  & 60.67      \\
     &      &    & XLM-R\textsubscript{Large}      & 92.85  & 92.04  & 91.50      \\ &      &    & XLM-R\textsubscript{Large}      & 71.38  & 67.78  & 67.67      \\
     &      &    & AraBERT & 91.76  & 91.12  & 91.00      \\  &      &    & AraBERT & 63.78  & 58.33  & 72.00      \\
     &      &    &      \ourmodel  & 93.12  & 92.25  & \textbf{92.00}   \\  &      &    & \ourmodel& 68.73  & 65.36  & \textbf{76.50}   \\
     &      &    & \newmodel  & 93.85  & 92.98  & \textbf{93.00}   \\    &      &    & \newmodel  & 71.02  & 67.34  & \textbf{78.00}   \\ 
\hline

\toprule
\multicolumn{7}{l}{\textsuperscript{$\star$} \newcite{obeid2020camel}, \textsuperscript{$\star\star$} \newcite{mageed-2020-aranet}, \textsuperscript{$\dagger$} \newcite{antoun2020arabert}} \\
\multicolumn{7}{l}{For all the other datasets we consider AraBERT  as SOTA.}
%     }\\     

% \newcite{obeid2020camel}, \textsuperscript{$\star\star$} \newcite{mageed-2020-aranet},   \textsuperscript{$\dagger$} \newcite{antoun2020arabert}.For all the other datasets we consider AraBERT model as SOTA.

\end{tabular}}\end{adjustbox}

\caption{\footnotesize{Sentiment Analysis Results. }}
\label{tab:senti_results}
\end{table*}
