# Supplementary material for: ARBERT & MARBERT: Deep Bidirectional Transformers for Arabic
Source: arXiv:2101.01785 source file (2021-06-07)
Supplement: Supplementary file 2 [file SM_tasks.tex]

\footnotesize
\begin{center}
\begin{table*}[ht]
\begin{tabular}   {p{3.7cm}cp{1.7 cm}p{1.1cm}cp{2.4cm}p{1.2cm}}

  \toprule
 \textbf{Authors }& \textbf{Task} & \textbf{Sources}&  \textbf{Data}  &\textbf{ Class } &\textbf{ Classes }    &\textbf{MSA/DI} \\
  \toprule

\newcite{alshehri2020understanding} &      Dangerous  & Twitter   & $4,445$ &   2 &  safe or not & MSA+DI  \\ %\hline
\newcite{al2020proceedings} &  Offensive &   Twitter& $10,000$  &   2 &  offensive or not  & MSA+DI\\ %\hline
\newcite{al2020proceedings} &   Hate & Twitter &  $10,000$   &   2 & hate or not & MSA+DI\\ %\hline
\newcite{farha2020arabic} & Sarcasm & Twitter &  $10,575$  &  2  & sarcasm or not& MSA+DI \\ %\hline
\newcite{farha2020arabic} & DI* & Twitter &  $10,575$  &  5  & sarcasm or not& MSA+DI \\ %\hline
\newcite{farha2020arabic} & SA* & Twitter &  $10,575$  & 3  & sarcasm or not& MSA+DI \\ %\hline
  \toprule
\end{tabular}
\caption{Social Meaning Tasks Datasets. }
\label{tab:sentiment}
\end{table*}
\end{center}
\normalsize
